# Supplementary material for: More Grounded Image Captioning by Distilling Image-Text Matching Model
Source: arXiv:2004.00390 source file (2020-04-01)
Supplement: Supplementary file 1 [file supple.tex]

% \documentclass[10pt,onecolumn,letterpaper]{article}

% \usepackage{cvpr}
% \usepackage{times}
% \usepackage{epsfig}
% \usepackage{graphicx}
% \usepackage{subcaption}
% \usepackage{amsmath}
% \usepackage{amssymb}
% \usepackage{bm}
% \usepackage{textcomp}
% \usepackage{enumitem}
% \usepackage{multirow}
% \renewcommand{\thefigure}{\Alph{figure}}
% \renewcommand{\thetable}{\Alph{table}}
% \renewcommand{\theequation}{\Alph{equation}}
% \renewcommand{\thesection}{\Alph{section}}

% % Include other packages here, before hyperref.

% % If you comment hyperref and then uncomment it, you should delete
% % egpaper.aux before re-running latex.  (Or just hit 'q' on the first latex
% % run, let it finish, and you should be clear).
% \usepackage[pagebackref=true,breaklinks=true,letterpaper=true,colorlinks,bookmarks=false]{hyperref}
% % \usepackage[breaklinks=true,bookmarks=false]{hyperref}

% \cvprfinalcopy % *** Uncomment this line for the final submission

% \def\cvprPaperID{****} % *** Enter the ICCV Paper ID here
% \def\httilde{\mbox{\tt\raisebox{-.5ex}{\symbol{126}}}}

% % Pages are numbered in submission mode, and unnumbered in camera-ready
% \ifcvprfinal\pagestyle{empty}\fi
% \setcounter{page}{1}
% \begin{document}

% %%%%%%%%% TITLE
% \title{Supplementary Material for ``Generating More Grounded Image Captions by Distilling Local Image-Text Matching Model''}

% \maketitle
% \thispagestyle{empty}

\section{Supplementary material}
\subsection{Quantitative results}
% \input{tables/sup_tab}

% we find that if $\lambda_{1}$ is set to $0.2$ when we use visual feature from   \cite{zhou2019grounded}, the  performance of \emph{Our\textsuperscript{\dag}}  can be further improved, as shown in Table \ref{sup_tab}.
We have also reported the caption evaluation results on MS-COCO \cite{lin2014microsoft} (cf. Table~\ref{mscoco}). Note that the implementation details remain the same except that we set LSTM hidden state size to $1024$ and train the model for  $30$ epochs in the second training stage with batch size $32$. During testing, we set the beam search size to $3$. We can see: first, compared to the baseline \cite{anderson2018bottom}, our method does not hurt the CIDEr score (slightly better) while improves the SPICE score by 0.6 point, the reason is that SPICE encourages visually grounded captions. However, since there is no straightforward  region-word alignment annotations in the MS-COCO captioning dataset, the main attention evaluation results are not available.

\subsection{Qualitative results}
In this section, we provide more qualitative results to demonstrate the benefits of our method. From Figure \ref{sup1}, we can observe that \emph{Up-Down+XE+0.1KL} model generates more grounded captions than \emph{Up-Down+XE} model. For example, \emph{Up-Down+XE+0.1KL} model correctly relates `man' and `woman' with corresponding regions but \emph{Up-Down+XE} model gets it backwards  in the bottom-right of Figure \ref{sup1}.  In Figure \ref{sup2}, though both models can well align words with regions, the captions generated by \emph{Up-Down+XE+0.1KL+1.0CIDEr+1.0Local} model are more faithful to image. For example, \emph{Up-Down+XE+0.1KL+1.0CIDEr+1.0Local} model further specifies  the `black wetsuit' worn by `surfer' in the bottom-right of Figure \ref{sup2}.

%---------------------------------------------------------------------------------------
\begin{table}[H]
\begin{center}
\setlength{\tabcolsep}{1mm}{
\begin{tabular}{|l|ccccc|}
\hline
\cline{2-6}
& B@1    & B@4    & M      & C      & S  \\ \hline \hline
UD+XE\textsuperscript{*}\cite{anderson2018bottom} & 77.2   & 36.2   & 27.0   & 113.5  & 20.3  \\
UD+XE+C\textsuperscript{*}\cite{anderson2018bottom} & 79.8   & 36.3   & 27.7   & 120.1  & 21.4  \\  \hline
UD+XE  & 76.2   & 36.4   & 27.7   & 113.1   & 20.5   \\
UD+XE+C & 80.0 & 37.8 & 28.1   & 125.2   & 21.6   \\
UD+XE+C+Local & 79.8 & 37.8 & 28.5 & \textbf{126.6}   & 22.2  \\ \hline
UD+XE+KL & 76.6 & 36.5 & 27.9   & 114.9   & 20.8   \\
UD+XE+KL+C & 80.1 & 37.8 & 28.3   & 125.9   & 22.0 \\
UD+XE+KL+C+Local & \textbf{80.2} & \textbf{38.0} & \textbf{28.5}   & 126.1  & \textbf{22.2}  \\  \hline
\end{tabular}}
\end{center}
\caption{Performance on the MS-COCO Karpathy test set. $*$ denotes results reported in the original paper. UD is short for Up-Down. Omitted balance weights equals to $1$. }
\label{mscoco}
% \vspace{-0.3cm}
\end{table}
%-----------------------------------------------------------------------------------

\begin{figure*}[t]
\begin{center}
%\fbox{\rule{0pt}{2in} \rule{0.9\linewidth}{0pt}}
   \includegraphics[width=0.8\linewidth]{figures/imgs/sup1.png}
\end{center}
   \caption{Generated captions and internal region-word alignments with comparison between  \emph{Up-Down+XE} and  \emph{Up-Down+XE+0.1KL}. In each unit, the image in the left and caption surrounded by green box is from Up-Down+XE+0.1KL model and others from Up-Down+XE model. Word and corresponding attended region with maximum weight are marked with the same color. We also visualize the attention weight distributions of some visually-groundable words on top of captions. The darker the color, the bigger the weight.}
\label{sup1}
\end{figure*}

\begin{figure*}[t]
\begin{center}
%\fbox{\rule{0pt}{2in} \rule{0.9\linewidth}{0pt}}
   \includegraphics[width=0.8\linewidth]{figures/imgs/sup2.png}
\end{center}
   \caption{Generated captions and internal region-word alignments with comparison between \emph{Up-Down+XE+0.1KL} and  \emph{Up-Down+XE+0.1KL+1.0CIDEr+1.0Local}. In each unit, the image in the left and caption surrounded by green box is from \emph{Up-Down+XE+0.1KL+1.0CIDEr+1.0Local} model and others from \emph{Up-Down+XE+0.1KL} model. Word and corresponding attended region with maximum weight are marked with the same color. We also visualize the attention weight distributions of some visually-groundable words on top of captions. The darker the color, the bigger the weight.}
\label{sup2}
\end{figure*}

% {\small
% \bibliographystyle{ieee_fullname}
% \bibliography{citations}
% }

% \end{document}
